# Supplementary material for: Long Story Short: Story-level Video Understanding from 20K Short Films
Source: arXiv:2406.10221 source file (2026-08-28)
Supplement: Supplementary file 1 [file checklist.tex]

%%%%%%%%%%%%%%%%%%%%%%%%%%%%%%%%%%%%%%%%%%%%%%%%%%%%%%%%%%%%
\section{Checklist}
\label{subsec:checklist}
\begin{comment}
%%% BEGIN INSTRUCTIONS %%%
The checklist follows the references.  Please
read the checklist guidelines carefully for information on how to answer these
questions.  For each question, change the default \answerTODO{} to \answerYes{},
\answerNo{}, or \answerNA{}.  You are strongly encouraged to include a {\bf
justification to your answer}, either by referencing the appropriate section of
your paper or providing a brief inline description.  For example:
\begin{itemize}
  \item Did you include the license to the code and datasets? \answerYes{See Section~\ref{gen_inst}.}
  \item Did you include the license to the code and datasets? \answerNo{The code and the data are proprietary.}
  \item Did you include the license to the code and datasets? \answerNA{}
\end{itemize}
Please do not modify the questions and only use the provided macros for your
answers.  Note that the Checklist section does not count towards the page
limit.  In your paper, please delete this instructions block and only keep the
Checklist section heading above along with the questions/answers below.
%%% END INSTRUCTIONS %%%
\end{comment}

% \begin{enumerate}

% \item For all authors...
% \begin{enumerate}
%   \item Do the main claims made in the abstract and introduction accurately reflect the paper's contributions and scope?
%     \answerYes{}
%   \item Did you describe the limitations of your work?
%     \answerYes{}
%   \item Did you discuss any potential negative societal impacts of your work?
%     \answerYes{See Supplementary Materials Section~\ref{subsec:ethical_considerations}}
%   \item Have you read the ethics review guidelines and ensured that your paper conforms to them?
%     \answerYes{See Supplementary Materials Section~\ref{subsec:ethical_considerations}}
% \end{enumerate}

% \item If you are including theoretical results...
% \begin{enumerate}
%   \item Did you state the full set of assumptions of all theoretical results?
%     \answerNA{}
% 	\item Did you include complete proofs of all theoretical results?
%     \answerNA{}
% \end{enumerate}

% \item If you ran experiments (e.g. for benchmarks)...
% \begin{enumerate}
%   \item Did you include the code, data, and instructions needed to reproduce the main experimental results (either in the supplemental material or as a URL)?
%     \answerYes{~\url{https://huggingface.co/datasets/rghermi/sfd}}
%   \item Did you specify all the training details (e.g., data splits, hyperparameters, how they were chosen)?
%     \answerYes{See Sections~\ref{subsec:baselines}, ~\ref{subsec:temporal_window_study}, and ~\ref{subsec:data_leakage}.}
% 	\item Did you report error bars (e.g., with respect to the random seed after running experiments multiple times)?
%     \answerNo{} Our experiments consist of benchmarking various aspects of our dataset. For a given compute, instead of performing one experiment several times (with different random seeds), we chose to experiment with several different multimodal methods and multiple LLMs. We observed that they all report similar performances and overall follow the same trend; hence, we argue that our findings are generalizable.
% 	\item Did you include the total amount of compute and the type of resources used (e.g., type of GPUs, internal cluster, or cloud provider)?
%     \answerYes{See Section~3.3}
% \end{enumerate}

% \item If you are using existing assets (e.g., code, data, models) or curating/releasing new assets...
% \begin{enumerate}
%   \item If your work uses existing assets, did you cite the creators?
%     \answerYes{See Section~\ref{subsec:ethical_considerations}.}
%   \item Did you mention the license of the assets?
%     \answerYes{See Section~\ref{subsec:ethical_considerations}.}
%   \item Did you include any new assets either in the supplemental material or as a URL?
%     \answerNA{}
%   \item Did you discuss whether and how consent was obtained from people whose data you're using/curating?
%     \answerYes{See Section~\ref{subsec:ethical_considerations}.}
%   \item Did you discuss whether the data you are using/curating contains personally identifiable information or offensive content?
%     \answerNA{
%     %See Section~\ref{subsec:ethical_considerations}.}%\XWC{do we really discuss this?
%     }
% \end{enumerate}

% \item If you used crowdsourcing or conducted research with human subjects...
% \begin{enumerate}
%   \item Did you include the full text of instructions given to participants and screenshots, if applicable?
%     \answerYes{See Section~\ref{subsec:human_study}.}
%   \item Did you describe any potential participant risks, with links to Institutional Review Board (IRB) approvals, if applicable?
%     \answerNA{}
%   \item Did you include the estimated hourly wage paid to participants and the total amount spent on participant compensation?
%     \answerNA{}
% \end{enumerate}

% \end{enumerate}

%%%%%%%%%%%%%%%%%%%%%%%%%%%%%%%%%%%%%%%%%%%%%%%%%%%%%%%%%%%%
