# Supplementary material for: Long Story Short: Story-level Video Understanding from 20K Short Films
Source: arXiv:2406.10221 source file (2026-08-28)
Supplement: Supplementary file 2 [file instruction_tuning_add_results.tex]

\begin{comment}
\begin{figure}[h]
    \centering
    \includegraphics[width=\linewidth]{data/it_size_ablation.pdf}
    \caption{\textbf{Effect of the training size on the instruction tuning of Llava-OneVision-0.5B trained on Multiple-Choice QA.} Note that the number of instruction samples is approximately 10x the number of videos.}
    \label{fig:it_size_ablation}
\end{figure}

\section{Instruction tuning additional results}
\label{subsec:instruction_tuning_add_results}

We report additional results from the instruction tuning experiment detailed in Section~4.6.

\noindent\textbf{Effect of the training size.} Figure~\ref{fig:it_size_ablation} shows the performance of Llava-OneVision-0.5B~\cite{li2024llavaonevisioneasyvisualtask} when instruction-tuned for multiple-choice question answering on SF20K-Train, with varying numbers of training videos. We subsample the full dataset at incremental values (70, 140, 281, 562, 1125, 2250, 4500, 9000, and 18,000 videos). Results indicate a logarithmic improvement in accuracy as the training set size increases, rising from 46.5\% to 63.0\%. Results are displayed in log-scale. These findings highlight the scalability benefits of instruction tuning on SF20K.

\noindent\textbf{Open-ended QA performance.} Table~\ref{tab:oeqa_it_perf} shows Llava-OneVision-0.5B~\cite{li2024llavaonevisioneasyvisualtask} performance on open-ended question answering after instruction tuning. 
%In details, we unify both multiple-choice and open-ended QA using a similar response format: "(X) [RESPONSE]" for multiple-choice QA and "[RESPONSE]".
Despite the being a much more complex task, we observe a modest overall improvement of +4.0\%.
\end{comment}

\begin{comment}
\begin{table}
    \label{}
    \centering
    \resizebox{1.0\columnwidth}{!}{
    \begin{tabular}{crcccc}
        \toprule
        \multirow{2}{*}{Fine-tuned} & \multirow{2}{*}{\#Videos} & \multicolumn{2}{c}{Multiple-Choice QA} & \multicolumn{2}{c}{Open-Ended QA} \\
        & & VL & $+\Delta$ & VL & $+\Delta$ \\
        \midrule
        \rxmark &      - & 37.8 & & 22.6 & \\
        \gcmark &     70 & 46.5 & \textcolor{my_green}{+8.7} & x & \textcolor{my_green}{+x} \\
        \gcmark &    140 & 49.6 & \textcolor{my_green}{+11.8} & x & \textcolor{my_green}{+x} \\
        \gcmark &    281 & 56.1 & \textcolor{my_green}{+18.3} & x & \textcolor{my_green}{+x} \\
        \gcmark &    562 & 58.5 & \textcolor{my_green}{+20.7} & x & \textcolor{my_green}{+x} \\
        \gcmark &  1,125 & 59.4 & \textcolor{my_green}{+21.6} & x & \textcolor{my_green}{+x} \\
        \gcmark &  2,250 & 60.0 & \textcolor{my_green}{+22.2} & x & \textcolor{my_green}{+x} \\
        \gcmark &  4,500 & 61.1 & \textcolor{my_green}{+23.3} & x & \textcolor{my_green}{+x} \\
        \gcmark &  9,000 & 61.1 & \textcolor{my_green}{+23.3} & x & \textcolor{my_green}{+x} \\
        \gcmark & 18,000 & 63.0 & \textcolor{my_green}{+25.2} & x & \textcolor{my_green}{+x} \\
        \bottomrule
    \end{tabular}
    }
    \caption{Llava-OneVision-0.5B}
\end{table}
\end{comment}

\begin{comment}
\begin{table}
    \label{}
    \centering
    \resizebox{1.0\columnwidth}{!}{
    \begin{tabular}{crcc}
        \toprule
        \multirow{2}{*}{Fine-tuned} & \multirow{2}{*}{\#Videos} & \multicolumn{2}{c}{Multiple-Choice QA} \\
        & & VL & $+\Delta$ \\
        \midrule
        \rxmark &      - & 37.8 & \\
        \gcmark &     70 & 46.5 & \textcolor{my_green}{+8.7} \\
        \gcmark &    140 & 49.6 & \textcolor{my_green}{+11.8} \\
        \gcmark &    281 & 56.1 & \textcolor{my_green}{+18.3} \\
        \gcmark &    562 & 58.5 & \textcolor{my_green}{+20.7} \\
        \gcmark &  1,125 & 59.4 & \textcolor{my_green}{+21.6} \\
        \gcmark &  2,250 & 60.0 & \textcolor{my_green}{+22.2} \\
        \gcmark &  4,500 & 61.1 & \textcolor{my_green}{+23.3} \\
        \gcmark &  9,000 & 61.1 & \textcolor{my_green}{+23.3} \\
        \gcmark & 18,000 & 63.0 & \textcolor{my_green}{+25.2} \\
        \bottomrule
    \end{tabular}
    }
    \caption{Llava-OneVision-0.5B}
\end{table}
\end{comment}
